# Supplementary material for: Differentiable Convex Polyhedra Optimization from Multi-view Images
Source: arXiv:2407.15686 source file (2024-07-22)
Supplement: Supplementary file 1 [file supp.tex]

% Redefine table numbering to be alphabetical
% \renewcommand{\thetable}{\Alph{table}}

% Redefine figure numbering to be alphabetical

\setcounter{page}{1}
% \maketitlesupplementary
\onecolumn

\begin{center}
  {\Large \bf {Differentiable Convex Polyhedra Optimization from Multi-view Images} \\
  \vspace{4mm}
-- Supplementary Materials --
}
\end{center}

\section{Compactness Analysis}
In this section, we present the properties of the reconstructed mesh through detailed numerical metrics. We provide the average counts of vertices, polygonal faces, and triangulated faces across each category from our reconstruction experiments. Notably, there appears to be a general correlation between the vertex and face counts of both the reconstructed and the original ground truth (GT) meshes. This observation underscores the efficiency and adaptability of our method.
\begin{table}

\centering
\resizebox{\linewidth}{!}{%
\addtolength{\tabcolsep}{4pt} 
  \begin{tabular}{l ccccc cc cccccc}
  \toprule  
  % \cmidrule(lr){2-5}
  % \cmidrule(lr){6-7}  
  % \cmidrule(lr){8-10}
  % \cmidrule(lr){11-13}
  % \cmidrule(lr){14-15}
  %   \cmidrule(lr){16-17}
   & Plane & Car & Chair & Lamp & Table & Sofa &  Telephone &  Vessel & Loudspeaker & Cabinet & Display & bench & Rifle  \\
  
  \midrule
  \bf \#Vertices & 541.6 & 453.6  & 269.78&548.78 & 188.14&229.74  & 182.62&307.88 &217.18 &190.6 &170.32 &230.92 &410.3\\
  \bf \#Polygons & 300.15 &257.99  & 166.21&305.48 &125.02 & 146.13 & 122.53&185.24 & 139.82&126.51 & 115.87&146.72 &236.76\\
  \bf \#Triangles & 1020.96  & 843.44 & 475.84&1034.52 &313.56 & 396.0 &302.32 &552.32 &370.96 &317.84 &278.32 & 398.48&756.64\\
  \midrule
  % \bf \#GT Vertices & 16275.79 & 36919.14 & 2553.49 & 6944.08& 1160.26 &5917.5 & 3124.05 & 20515.61 & 3986.82 & 1879.29 &1326.28  & 4381.28& 6108.17\\
    \bf \#GT Vertices & 16K & 37K & 2.6K & 7K & 1.1K & 6K & 3.1K & 21K & 4K & 1.9K & 1.3K  & 4.4K& 6.1K\\
  \bottomrule
  \end{tabular}
}
  \caption{Reconstructed mesh property, here we show the average number of vertices, average number of polygons, and average number of triangulated faces of each category.}
\label{tab:nvdiffrec}
\end{table}

\section{Runtime Efficiency}
In this section, we examine the run time and memory usage in relation to varying numbers of convex polyhedra and hyperplanes.
\begin{table}

\centering
\resizebox{\linewidth}{!}{%
\addtolength{\tabcolsep}{8pt} 
  \begin{tabular}{l ccccc cc cccc}
  \toprule  
  % \cmidrule(lr){2-5}
  % \cmidrule(lr){6-7}  
  % \cmidrule(lr){8-10}
  % \cmidrule(lr){11-13}
  % \cmidrule(lr){14-15}
  %   \cmidrule(lr){16-17}
   & \bf \#Convexes & 1 & 2 & 4 & 8 & 16 &  32 &  64 & 128 & 256 & 512  \\
  
  \midrule
  \bf \#Planes 8 & \bf Time(Sec)    & 0.02 & 0.02 & 0.02 & 0.02 & 0.02 & 0.02 & 0.03 & 0.03 & 0.05 & 0.09\\
                 & \bf Memory (MB) & 0.5 & 0.5 & 0.5 & 0.5 & 0.8 & 0.8 & 0.8 & 1.0 &  1.8 & 3.0 \\
  \midrule
  \bf \#Planes 16 & \bf Time(Sec)    & 0.02 & 0.02 & 0.02 & 0.02 & 0.02 & 0.03 & 0.04 & 0.06 & 0.1 & 0.16\\
                 & \bf Memory (MB) & 0.5 & 0.5 & 0.5 & 0.5 & 0.8 & 1.0 & 1.2 & 2.0 & 3.8  & 7.0\\
  \midrule
  \bf \#Planes 32 & \bf Time(Sec)    & 0.02 & 0.02 & 0.02 & 0.02 & 0.03 & 0.04 & 0.05 & 0.1 & 0.17 & 0.33\\
                 & \bf Memory (MB) & 0.5 & 0.8 & 0.8 & 0.8 & 1.0 & 1.2 & 2.2 & 3.8 & 7.5 & 14.5\\
  \midrule
  \bf \#Planes 64 & \bf Time(Sec)    & 0.02 & 0.02 & 0.02 & 0.03 & 0.04 & 0.06 & 0.1 & 0.17 & 0.33 & 0.66\\
                 & \bf Memory (MB) & 0.8 & 0.8 & 1.2 & 1.0 & 1.2 & 2.2 & 4.2 & 7.8 & 15.0  & 29.8\\
  \midrule
  \bf \#Planes 128 & \bf Time(Sec)    & 0.02 & 0.03 & 0.04 & 0.05 & 0.06 & 0.09 & 0.17 & 0.33 & 0.66 & 1.31\\
                 & \bf Memory (MB) & 1.0 & 1.0 & 1.2 & 1.5 & 2.5 & 4.2 & 7.8 & 15.2 & 30.2 & 60\\
  \midrule
  \bf \#Planes 256 & \bf Time(Sec)    & 0.02 & 0.027 & 0.036 & 0.054 & 0.98 & 0.18 & 0.34 & 0.64 & 1.28 & 2.61\\
                 & \bf Memory (MB) & 1.2 & 1.5 & 1.8 & 2.5 & 4.2 & 7.8 & 15.2 & 30.2 & 60.5 & 120.6\\
  \midrule
  \bottomrule
  \end{tabular}

}
\caption{Runtime information about our method, in particular, we show speed and memory usage w.r.t different number of convex polyhedra and hyperplanes.}
\label{tab:nvdiffrec}
\end{table}

\begin{figure}[ht]
    \centering
    \includegraphics[width=0.98\textwidth]{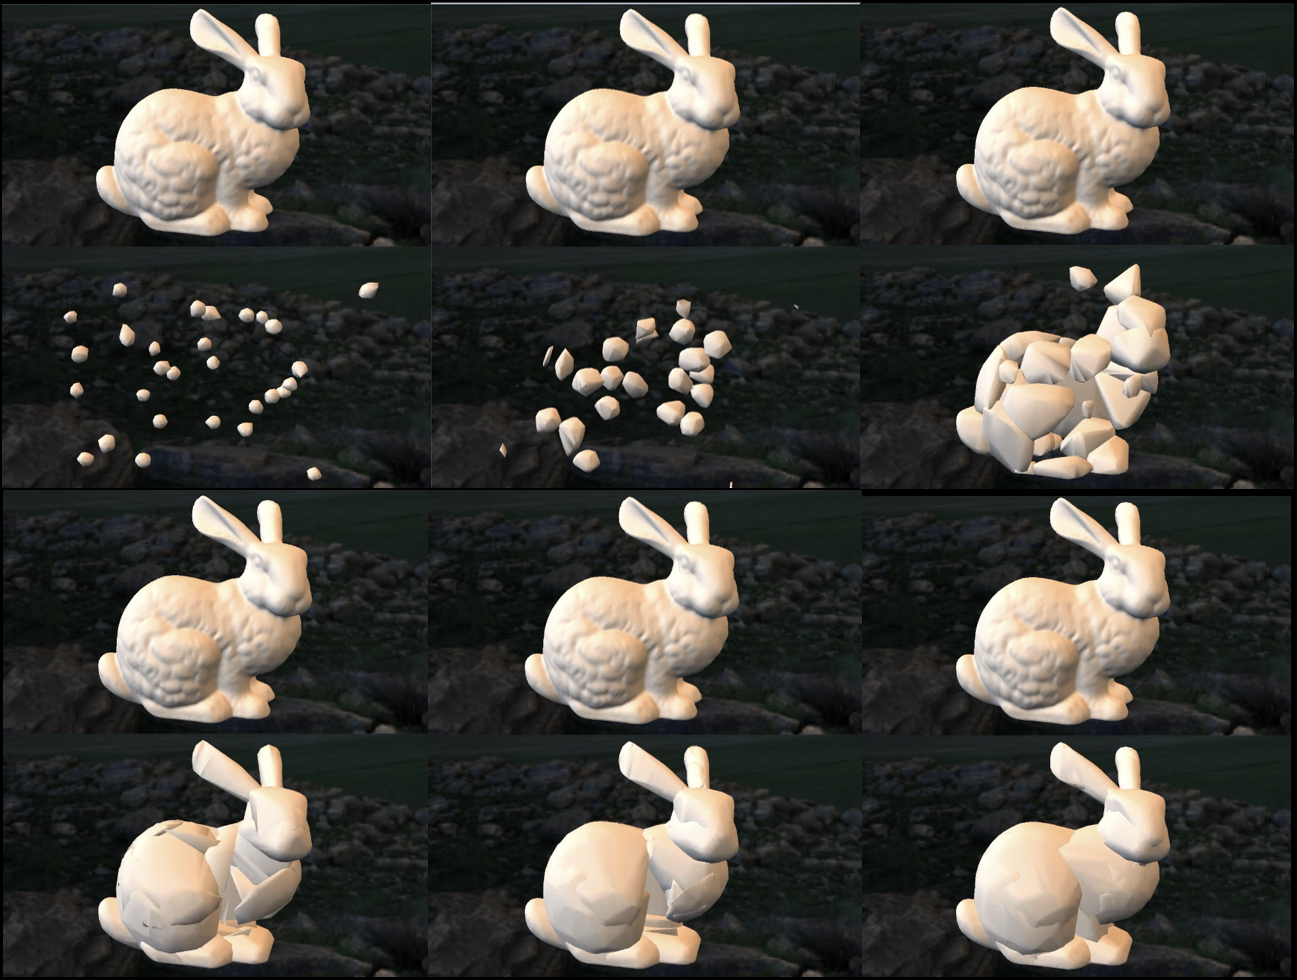}
    \caption{Screenshots from the attached video. \textbf{Row 1, 3:} Ground truth mesh. \textbf{Row 2, 4:} Optimized mesh.}
    \label{fig:overview}
\end{figure}

\section{Visulization of optimization Process}
We've included a video showcasing the optimization process for reconstructing a bunny from multiple viewpoints. The convex polyhedra begin in a random arrangement. Roughly every 10 seconds, operations for densification and convex spawning take place. The procedure utilizes a total of 32 convex polyhedra and undergoes 10,000 iterations.

\section{File Format}
To enhance the efficiency of storing, loading, and sharing shapes represented as convex polyhedra, we've developed a .cvx file format, reminiscent of .obj files. Each line in this format specifies a unique geometric entity. A 'p' at the beginning of a line identifies a hyperplane, accompanied by the components of its normal vector (nx, ny, nz) and the plane offset. Lines that start with 'c' indicate a convex polyhedron, defined by the indices of intersecting hyperplanes. The 't' character signals a translation of a convex polyhedron, directly linked to the polyhedron defined by the preceding 'c' lines. This data structure, also utilized in the optimization of convex polyhedra, proves to be extremely versatile, facilitating various operations such as densification, spawning, and removal.

The example below demonstrates how a .cvx file defines two cubes, each with a size of 2, and centers that are spaced 4 units apart.
\begin{lstlisting}[]
p  0  0  1  1
p  0  0 -1  1
p  0  1  0  1
p  0 -1  0  1
p  1  0  0  1
p -1  0  0  1
p  0  0  1  1
p  0  0 -1  1
p  0  1  0  1
p  0 -1  0  1
p  1  0  0  1
p -1  0  0  1
c  0  1  2  3  4  5
c  6  7  8  9 10 11 
t  0.0  0.0  0.0
t  4.0  0.0  0.0
\end{lstlisting}
